# Supplementary material for: GenSim: Generating Robotic Simulation Tasks via Large Language Models
Source: arXiv:2310.01361 source file (2024-01-21)

# RGB-D Input

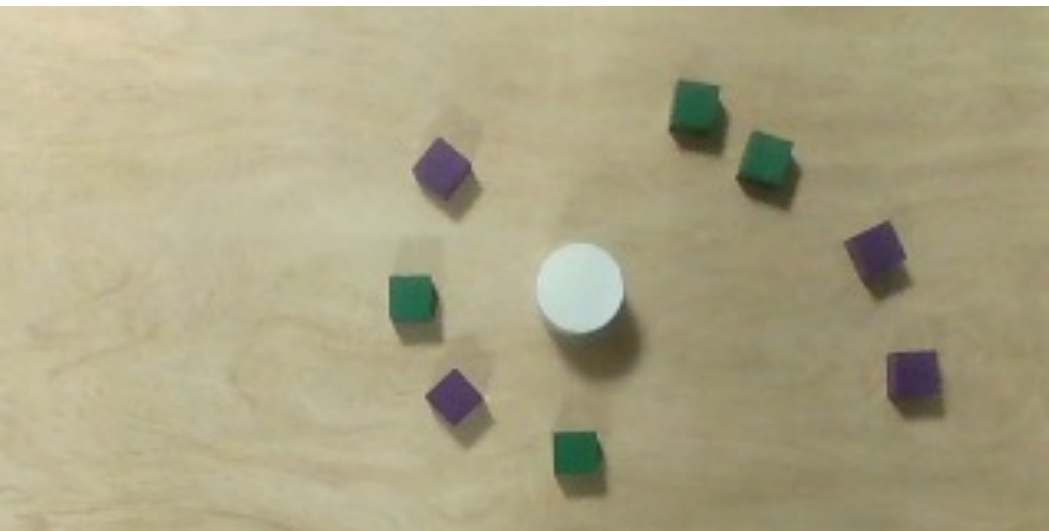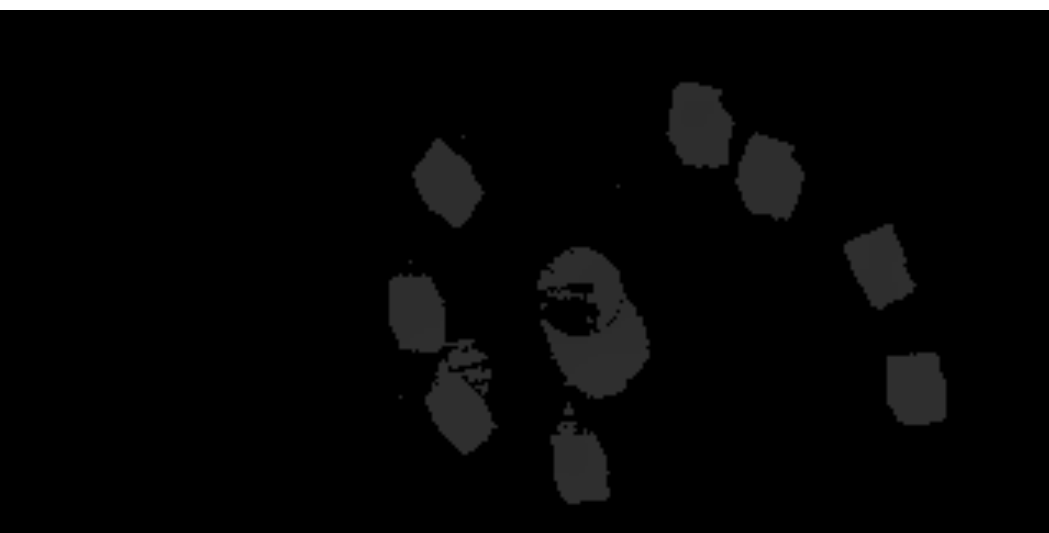

camera

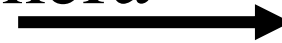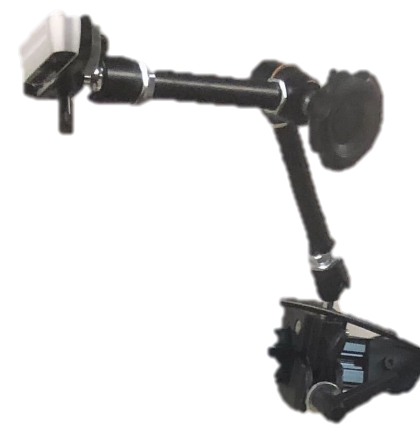

F/T sensor

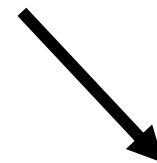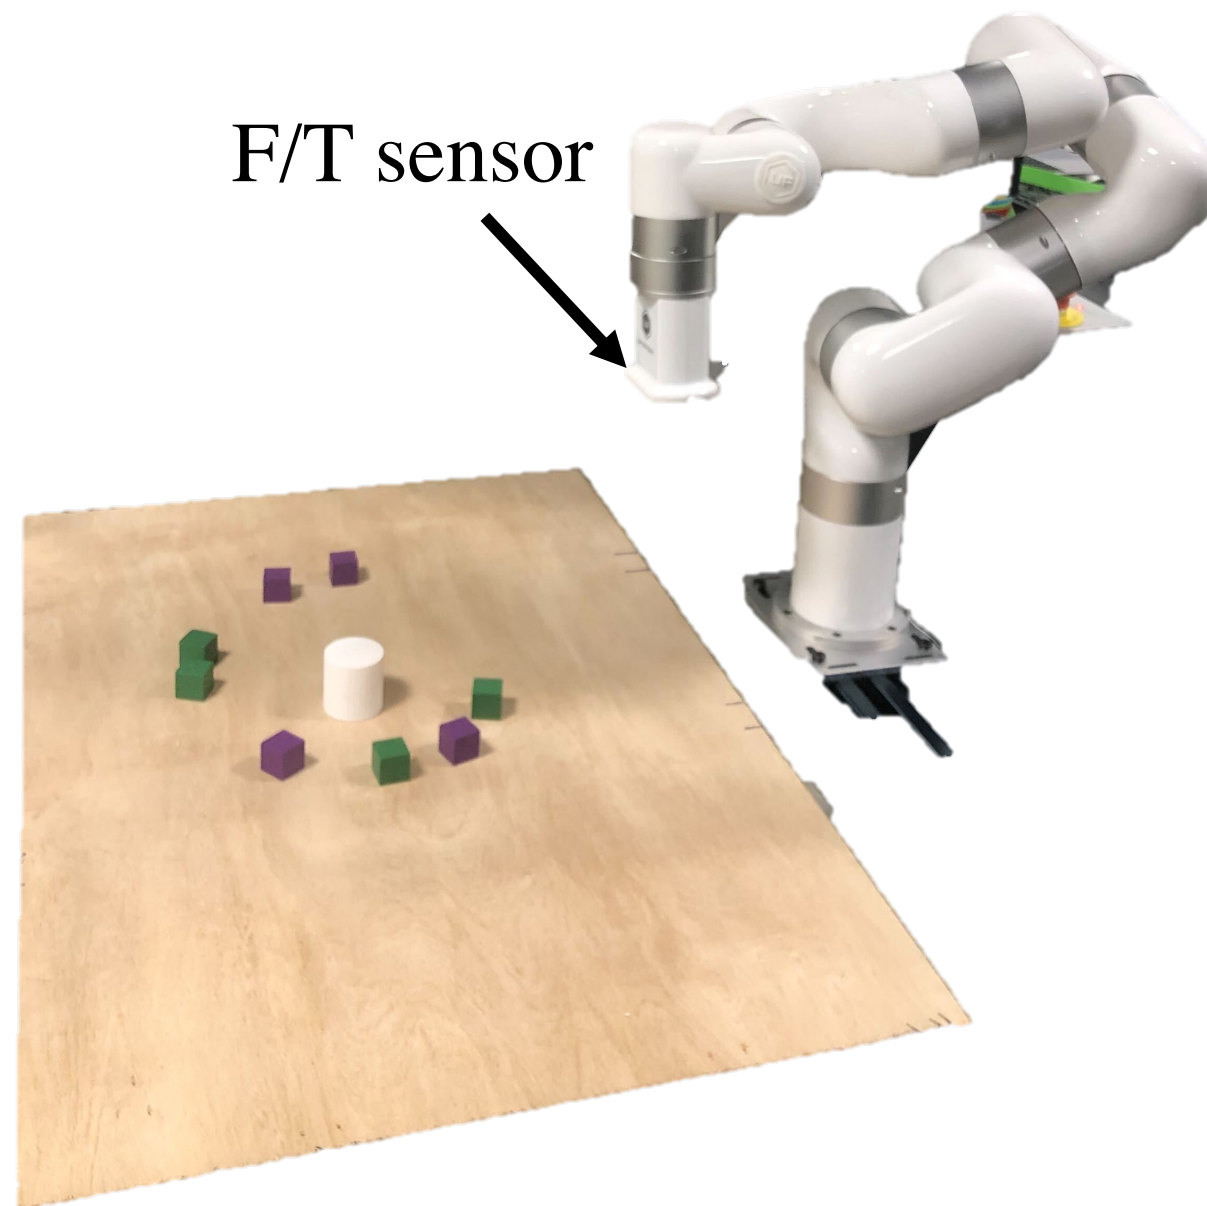



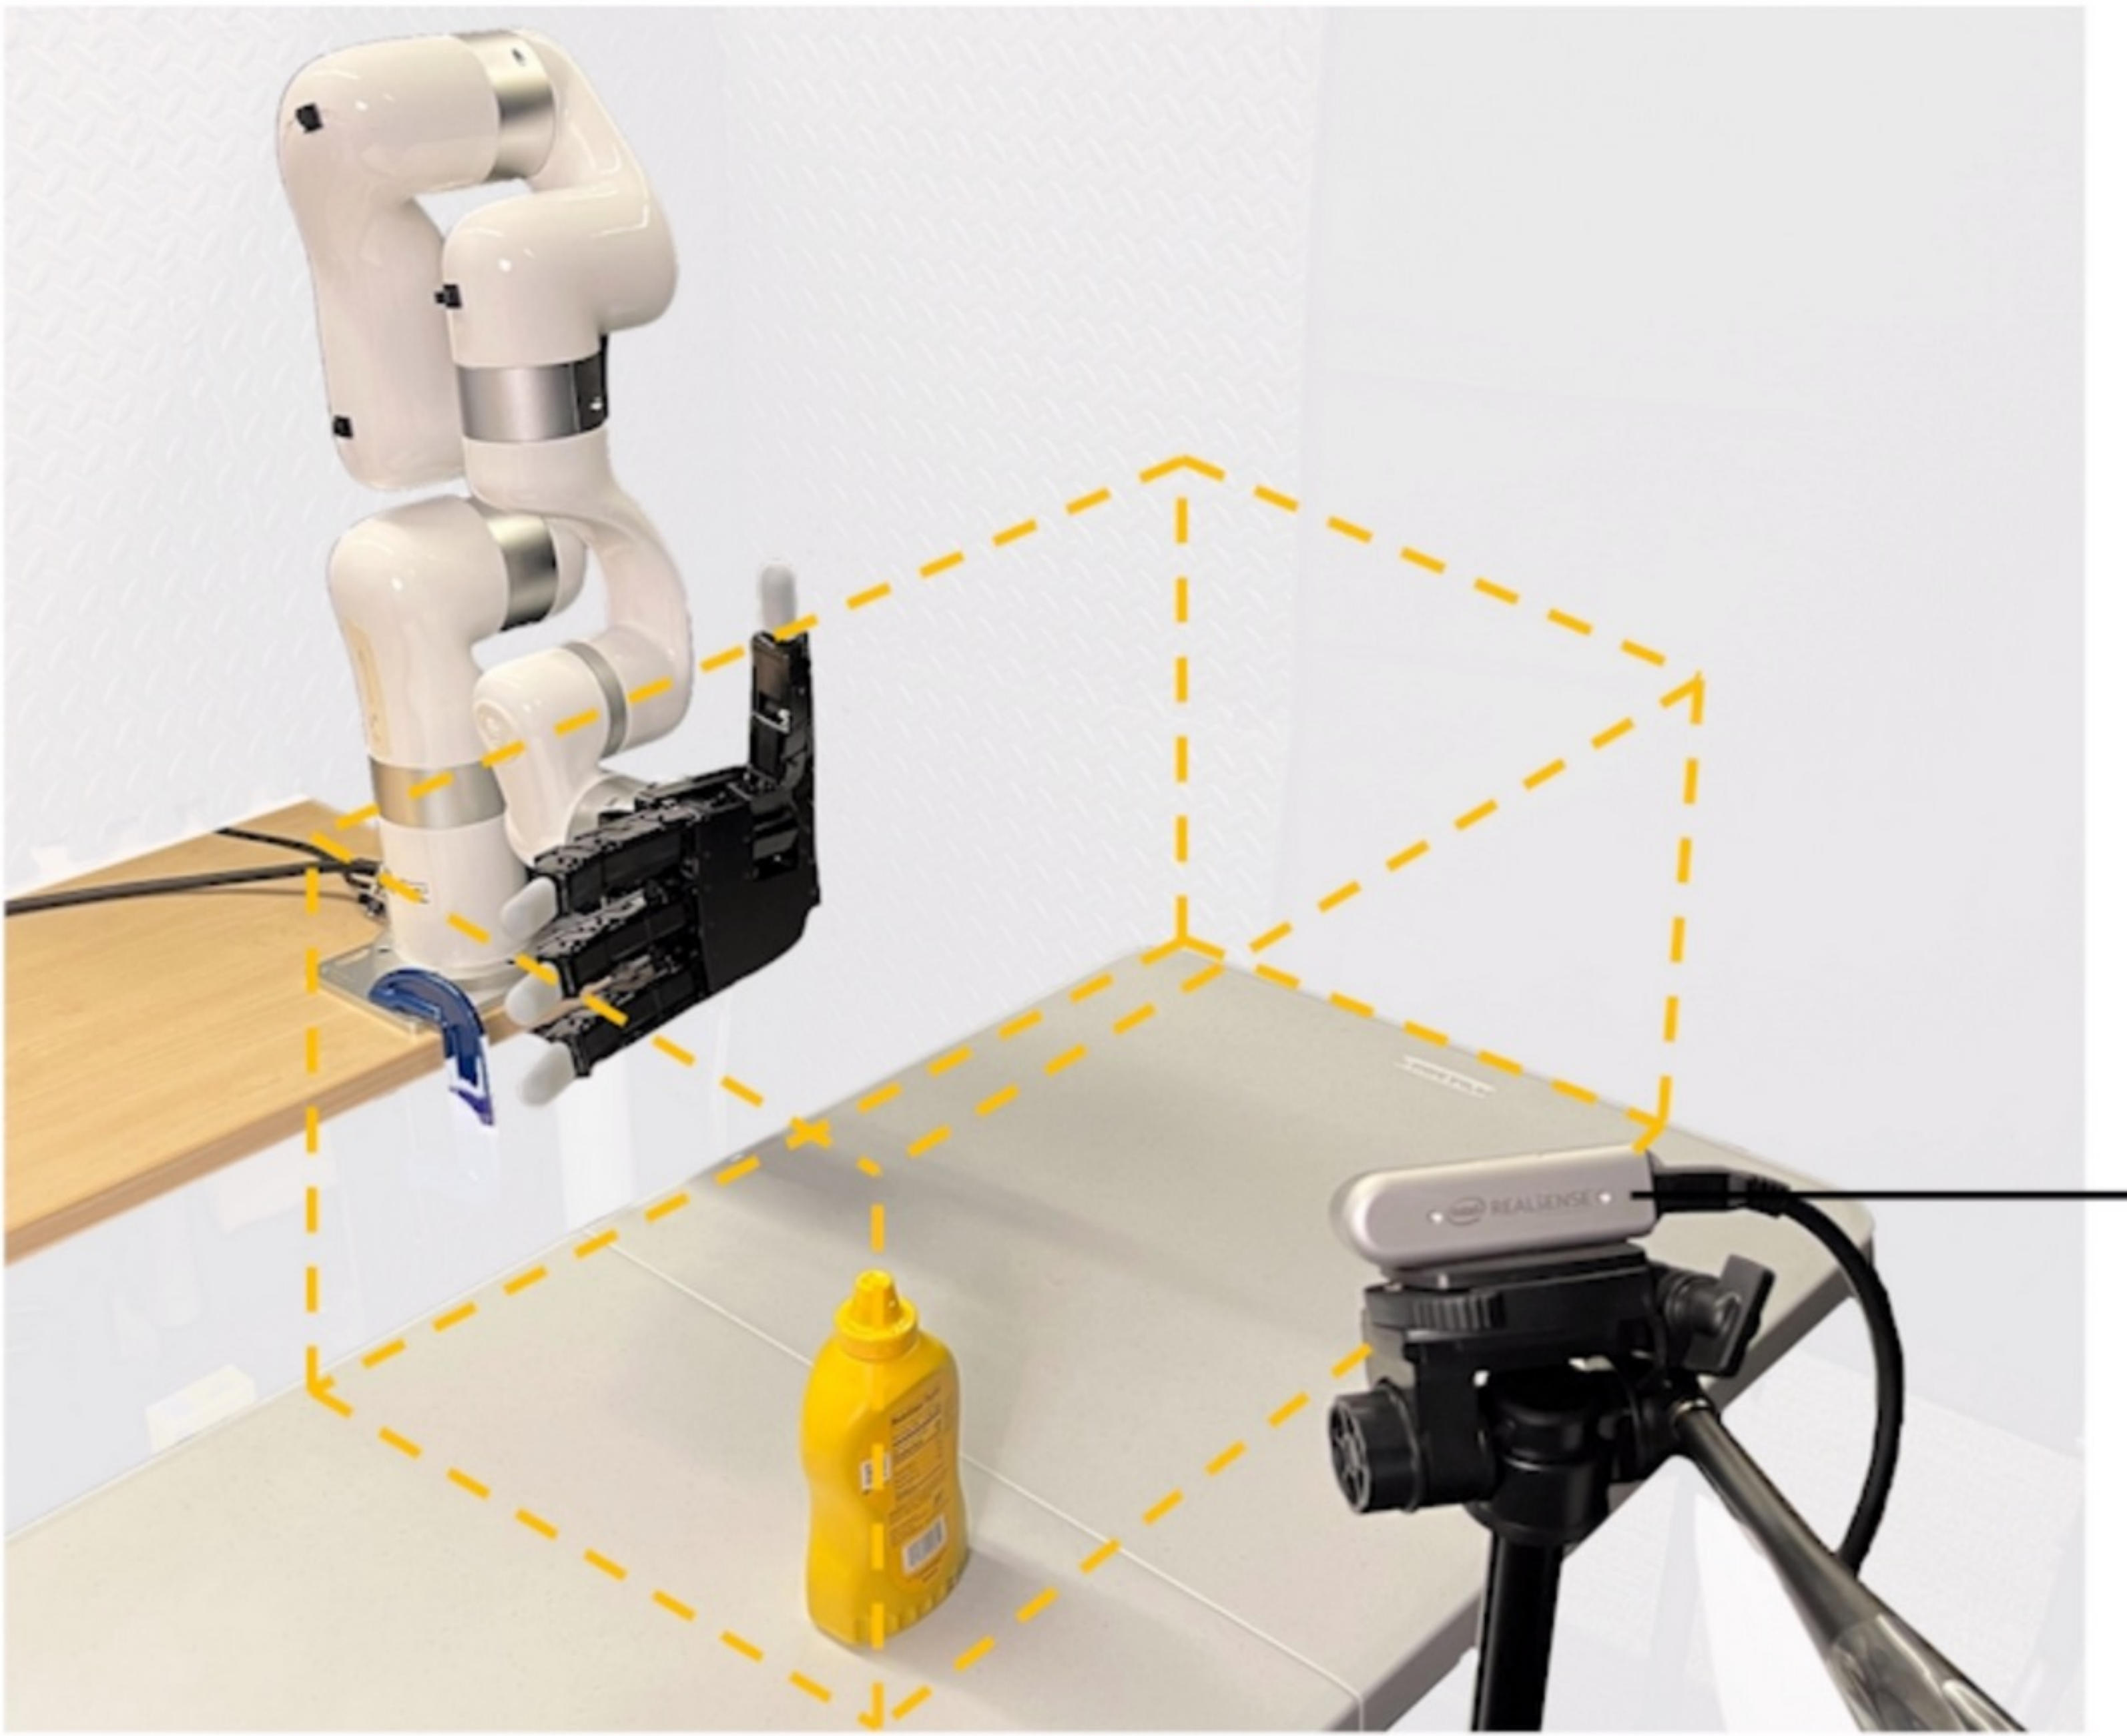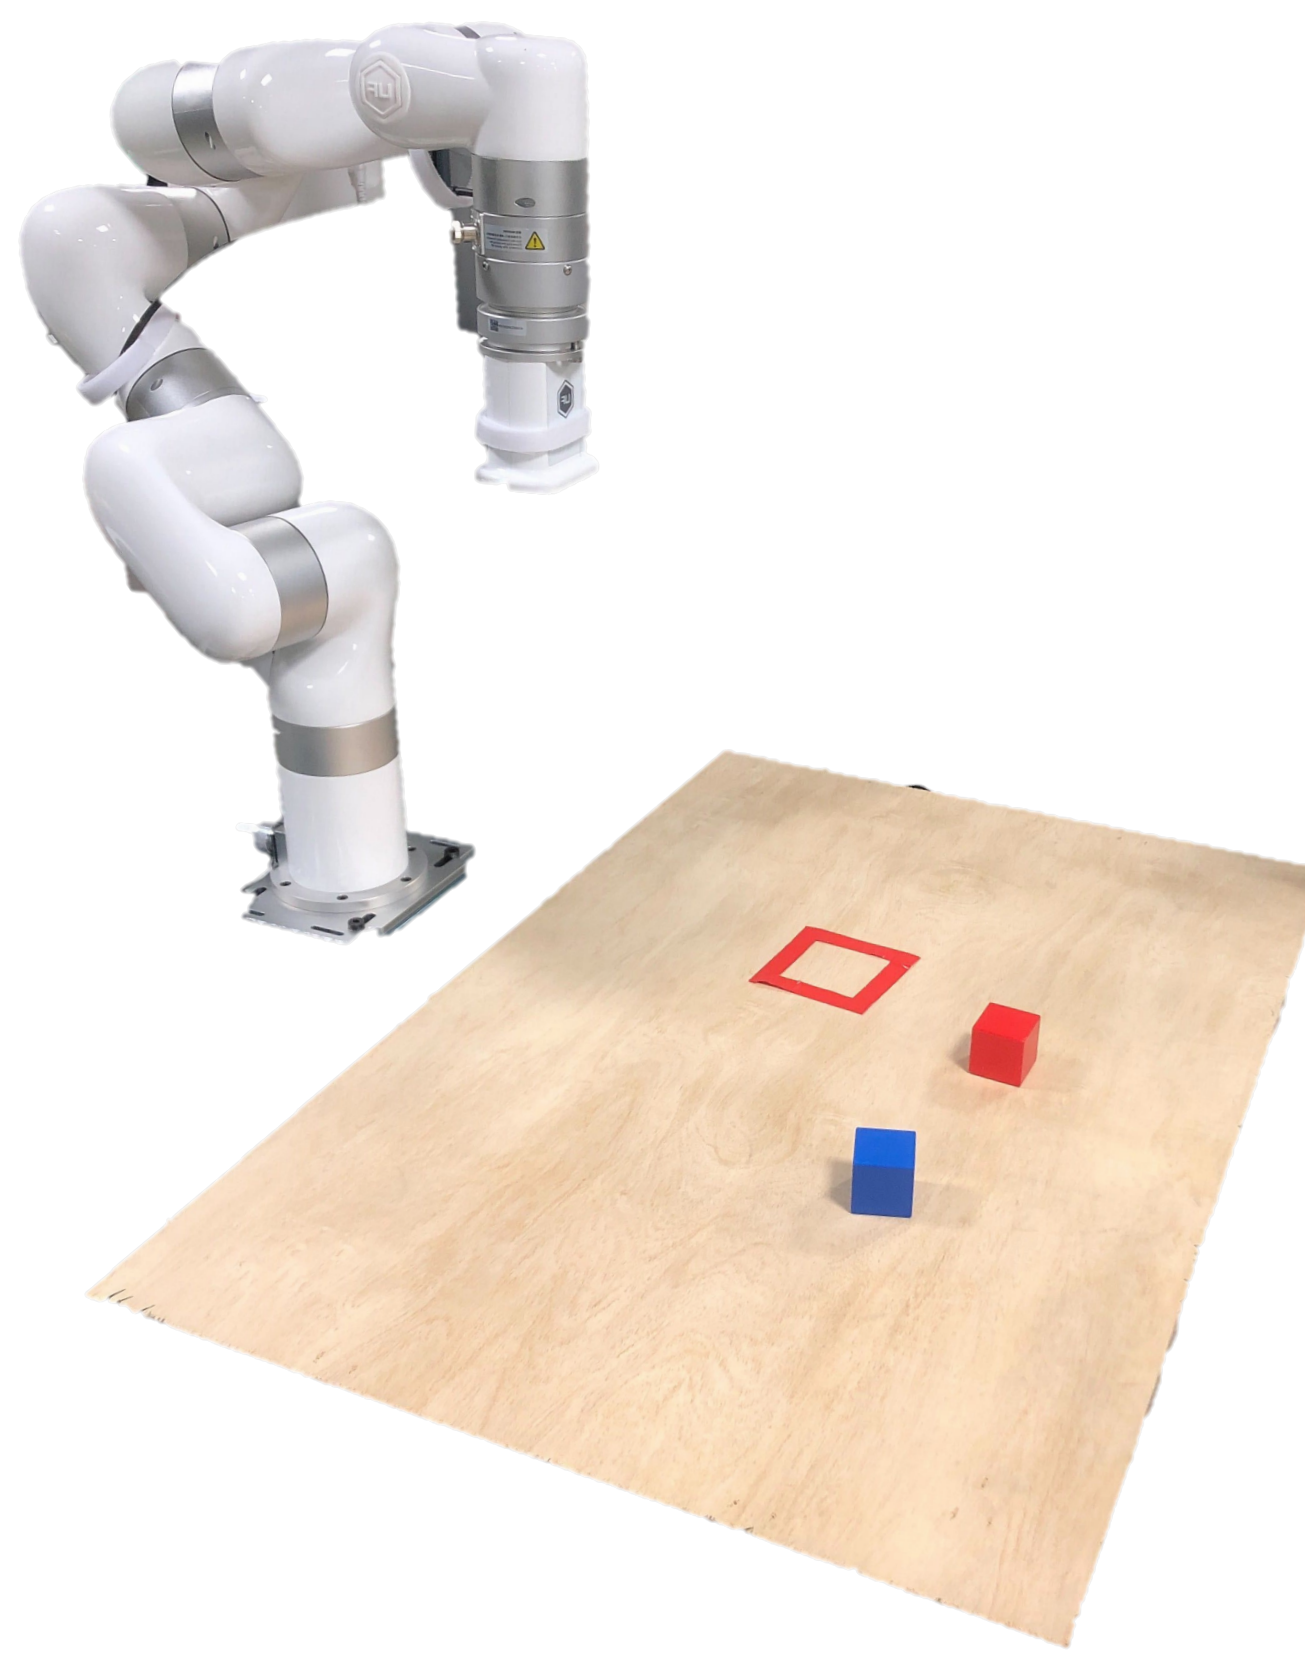

Supplement: Supplementary file 1 [file realworld_setup_appendix.pdf]
